# Supplementary material for: Global Convergence of Policy Gradient Methods to (Almost) Locally Optimal Policies
Source: arXiv:1906.08383 source file (2020-06-28)
Supplement: Supplementary file 1 [file Appendix_Lemmas.tex]

%!TEX root = Policy_Grad.tex
%%%%%%%%%%%%%%%%%%%%%%%%%%%%%%%%%%%%%%%%%%%%%%%%%%%%%%%%%%%%%%%%%%%%%%%%%%%%%
%%%%%%%%%%%%%%%%%%%%%%%%%%%%%%%%%%%%%%%%%%%%%%%%%%%%%%%%%%%%%%%%%%%%%%%%%%%%%%%%%%%%%%%%%%%%%%%% S  E  C T  I  O  N%%%%%%%%%%%%%%%%%%%%%%%%%%%%%%%%%%%%%%%%%%%%%%%%%%%%%%%%%%%%%%%%%%%%%%%%%%%%%%%%%%%%%%%%%%%%%%%%%%%%%%%%%%%%%%%%%%%%%%%%%%%%%%%%%%%%%%%%%%%%%%%%%%%%%%%%%%%%%%%%%%%%%%%%%%%%%%%%%%%%%%%%%%%%%%%%%%%%%%%%%%%
\clearpage
\appendix 

\section{Technical Lemmas}\label{append:lemmas}
In this section, we summarize all the technical lemmas used in the main text, whose proofs are deferred to \S\ref{append:proof}.
